# Supplementary material for: JSRehab: Weaning Common Web Interface Components from JavaScript Addiction
Source: arXiv:2203.06955 source file (2022-03-14)
Supplement: Supplementary file 1 [file appendix.tex]

\newpage
\section*{Appendix}

\begin{figure}[H]
  \centering
  \includegraphics[width=.7\linewidth]{bootstrap_component_share.pdf}
  \caption{Usage of \bootstrap{} components; Accordion and Offcanvas have only been introduced with \bootstrap{}~5, which has not yet been widely adopted.}\label{fig:bootstrap-component-usage}
\end{figure}

\begin{figure}[H]
  \centering
  \includegraphics[width=0.9\linewidth]{bootstrap_ranking_cdf.pdf}
  \caption{CDF of \tranco{} websites using \bootstrap{}'s \javascript{}.
  Usage of \bootstrap{}'s \javascript{} is uniform across website ranking, except for the very best ranked websites.}\label{fig:bootstrap-ranking-cdf}
\end{figure}

\begin{figure}[H]
  \caption{Example \texttt{webpack.config.js}}\label{fig:webpack-config-file}
  \lstinputlisting[
    style=javascript,
    language=C,
    ]{webpack-configuration.js}
\end{figure}

\input{bootstrap-components}

\begin{figure}[H]
  \centering
  \includegraphics[width=\linewidth]{bootstrap_versions.pdf}
  \caption{Versions of \bootstrap{}'s \javascript{} in use on crawled webpages; known vulnerable versions are marked with a *}\label{fig:bootstrap-versions}
\end{figure}
